# Supplementary material for: Local embedding of Coupled Cluster theory into the Random Phase Approximation using plane-waves
Source: arXiv:2012.06165 source file (2020-12-11)
Supplement: Supplementary file 1 [file supplemental.pdf]

# SUPPLEMENTARY MATERIAL FOR THE ARTICLE
# Local embedding of Coupled Cluster theory into the Random Phase Approximation using plane-waves

Tobias Schäfer, Florian Libisch, Georg Kresse, and Andreas Grüneis

## CONTENTS

I. PAW pseudo potentials 3

II. Compression of the unoccupied space 3

III. Computing the optimized auxiliary field 3

IV. Atomic structures of all benchmark systems 4
- A. $H_2O$@$h$-BN (far) 4
- B. $H_2O$@$h$-BN (int) 5
- C. $CH_4$ in chabazite crystal 7
- D. $H_2O$@$TiO_2$ (far) 8
- E. $H_2O$@$TiO_2$ (int, unrelaxed) 10
- F. $H_2O$@$TiO_2$ (int, relaxed using DFT-PBE) 13
- G. NaCl pristine cell 16
- H. NaCl with Na impurity (relaxed using DFT-PBE) 20

References 24

## I. PAW PSEUDO POTENTIALS

In the following table, we list the explicitly treated valence electrons, core radii $r_C$, and default energy cutoffs ENMAX for the PAW potentials:

| Element | Valence | $r_C$ (Å) | ENMAX (eV) |
|---|---|---|---|
| H | $1s^1$ | 1.10 | 300.000 |
| Li | $2s^1$ | 2.10 | 112.104 |
| B | $2s^2\ 2p^1$ | 1.70 | 318.614 |
| C | $2s^2\ 2p^2$ | 1.60 | 413.992 |
| N | $2s^2\ 2p^3$ | 1.60 | 420.902 |
| O | $2s^2\ 2p^4$ | 1.60 | 434.431 |
| Na | $2p^6\ 3p^1$ | 2.20 | 372.853 |
| Al | $3s^2\ 3p^1$ | 2.00 | 240.300 |
| Si | $3s^2\ 3p^2$ | 1.90 | 245.345 |
| Cl | $3s^2\ 3p^5$ | 1.90 | 262.472 |
| Ti | $3s^2\ 3p^6\ 3d^4$ | 2.00 | 383.774 |

## II. COMPRESSION OF THE UNOCCUPIED SPACE

The aim of constructing compact unoccupied orbitals in the present work is to find an unoccupied orbital manifold that can be used for the efficient calculation of dynamic correlation energies for a set of localized occupied orbitals. In this work the canonical virtual HF orbitals for the full supercell calculation form the starting point of the subsequent two-step orbital transformation procedure. First we compute the RPA natural orbitals (RPANOs) for the entire supercell prior to the localization procedure of the occupied orbitals. We restrict to the virtual-virtual ($N_\mathrm{v} \times N_\mathrm{v}$) block of the RPA reduced density matrix, leaving the occupied block untouched. We truncate the RPANOs to a subset constructed from $X$ (usually $X = 40, .., 60$) natural orbitals per occupied spatial orbital and recanonicalize the Fock matrix in this subspace. We refer to the corresponding total number of unoccupied orbitals at this stage by $N_v^\mathrm{pre}$. In the second compression step we compute approximate MP2 natural orbitals for a set of localized occupied orbitals. To this end we calculate the virtual-virtual ($N_\mathrm{v}^\mathrm{pre} \times N_\mathrm{v}^\mathrm{pre}$) block of an approximate MP2 reduced density matrix defined by Eq.2 in Ref. [1]. In this step the sum over the occupied orbitals for the expression of the reduced density matrix is restricted to a set of semi-canonicalized occupied orbitals that are localized on the fragment. As a consequence, the resulting approximate MP2NOs with the largest occupation numbers are also localized on the fragment. We refer to the corresponding number of employed NOs by $N_\mathrm{v}^\mathrm{loc}$. Although a simple one-step procedure would yield identical results, we choose to employ a two-step procedure to maximize the computational efficiency.

## III. COMPUTING THE OPTIMIZED AUXILIARY FIELD

As outlined in Ref. [2], we compute all Coulomb integrals, $V_{sr}^{pq}$, needed by CCSD theory from the Coulomb vertex $\Gamma{*}_s^{pG}$ using the following expression

$$V_{sr}^{pq} = \sum_{G=1}^{N_G} \Gamma{*}_s^{pG} \Gamma_{rG}^{q}, \quad (1)$$

where $p, q, r$ and $s$ refer to orbital indices. $G$ refers to auxiliary plane wave basis functions that are used to expand the densities of the orbital pairs $s$, $p$ and $q$, $r$. Furthermore we note that each Coulomb vertex includes a factor that corresponds to the square root of the Coulomb kernel in reciprocal space. For the outlined algorithm, the Coulomb vertex is computed after all orbitals have been compressed and are localized on the defined fragment. Therefore it is possible to take advantage of the optimized auxiliary field algorithm outlined in Ref. [2] and compress the number of plane wave basis functions $N_G$ used to expand the pair densities of the localized orbitals as well. To this end we perform a singular value decomposition of the $N_G \times N_G$ matrix defined by Eq.10 in Ref. [2] and truncating singular vectors that correspond to small singular values. The truncated singular vectors are then used to transform the $G$-index of the Coulomb vertex to the optimized auxiliary field basis. For the present work, significant reductions of the auxiliary basis set size are possibly without compromising the precision of computed correlation energies. We have carefully checked that the computed correlation energies are converged to within meV with respect to the size of the optimized auxiliary basis set.

## IV. ATOMIC STRUCTURES OF ALL BENCHMARK SYSTEMS

In the following we list all POSCAR files as used in VASP to define the atomic species and positions. We also provide the Hartree-Fock energy obtained with the used pseudo potential as described in in Sec. I.

### A. $H_2O$@*h*-BN (far)

Hartree-Fock energy: −1126.760 eV.

```
H2O@hBN (far)
1.0
        15.0714654922          0.0000000000          0.0000000000
        -7.5357344841         13.0522709851          0.0000000000
         0.0000000000          0.0000000000         16.0000000000
 H  O  N  B
 2  1  36  36
Cartesian
      1.83595549          3.82563121          8.520000000
      1.32595549          3.65563121          7.070000000
      1.05595549          3.55563121          8.000000000
      2.511910677         1.450252175         0.000000000
      1.255954862         3.625631094         0.000000000
     -0.000000873         5.801009178         0.000000000
     -1.255956531         7.976387501         0.000000000
     -2.511912584        10.151766777         0.000000000
     -3.767868042        12.327144623         0.000000000
      5.023821831         1.450252175         0.000000000
      3.767865658         3.625631094         0.000000000
      2.511909962         5.801009178         0.000000000
      1.255954385         7.976387501         0.000000000
     -0.000001583        10.151766777         0.000000000
     -1.255957007        12.327144623         0.000000000
      7.535732746         1.450252175         0.000000000
      6.279776573         3.625631094         0.000000000
      5.023820877         5.801009178         0.000000000
      3.767865181         7.976387501         0.000000000
      2.511909246        10.151766777         0.000000000
      1.255953908        12.327144623         0.000000000
     10.047642708         1.450252175         0.000000000
      8.791687012         3.625631094         0.000000000
      7.535731316         5.801009178         0.000000000
      6.279775620         7.976387501         0.000000000
      5.023819923        10.151766777         0.000000000
      3.767864227        12.327144623         0.000000000
     12.559554100         1.450252175         0.000000000
     11.303598404         3.625631094         0.000000000
     10.047642708         5.801009178         0.000000000
      8.791687012         7.976387501         0.000000000
      7.535731316        10.151766777         0.000000000
      6.279775620        12.327144623         0.000000000
      0.000000255         1.450252175         0.000000000
     -1.255955696         3.625631094         0.000000000
     -2.511911392         5.801009178         0.000000000
     -3.767867088         7.976387501         0.000000000
     -5.023822784        10.151766777         0.000000000
     -6.279778481        12.327144623         0.000000000
      0.000000000         0.000000000         0.000000000
```

| | | |
|---|---|---|
| −1.255955815 | 2.175378561 | 0.000000000 |
| −2.511911631 | 4.350757122 | 0.000000000 |
| −3.767867327 | 6.526135445 | 0.000000000 |
| −5.023823261 | 8.701514244 | 0.000000000 |
| −6.279778957 | 10.876892090 | 0.000000000 |
| 2.511910915 | 0.000000000 | 0.000000000 |
| 1.255955100 | 2.175378561 | 0.000000000 |
| −0.000000711 | 4.350757122 | 0.000000000 |
| −1.255956411 | 6.526135445 | 0.000000000 |
| −2.511912346 | 8.701514244 | 0.000000000 |
| −3.767867804 | 10.876892090 | 0.000000000 |
| 5.023821831 | 0.000000000 | 0.000000000 |
| 3.767866135 | 2.175378561 | 0.000000000 |
| 2.511910200 | 4.350757122 | 0.000000000 |
| 1.255954504 | 6.526135445 | 0.000000000 |
| −0.000001421 | 8.701514244 | 0.000000000 |
| −1.255956888 | 10.876892090 | 0.000000000 |
| 7.535732746 | 0.000000000 | 0.000000000 |
| 6.279777050 | 2.175378561 | 0.000000000 |
| 5.023821354 | 4.350757122 | 0.000000000 |
| 3.767865419 | 6.526135445 | 0.000000000 |
| 2.511909485 | 8.701514244 | 0.000000000 |
| 1.255954027 | 10.876892090 | 0.000000000 |
| 10.047643661 | 0.000000000 | 0.000000000 |
| 8.791687965 | 2.175378561 | 0.000000000 |
| 7.535732269 | 4.350757122 | 0.000000000 |
| 6.279776573 | 6.526135445 | 0.000000000 |
| 5.023820400 | 8.701514244 | 0.000000000 |
| 3.767864943 | 10.876892090 | 0.000000000 |
| 12.559554100 | 0.000000000 | 0.000000000 |
| 11.303598404 | 2.175378561 | 0.000000000 |
| 10.047642708 | 4.350757122 | 0.000000000 |
| 8.791687012 | 6.526135445 | 0.000000000 |
| 7.535730839 | 8.701514244 | 0.000000000 |
| 6.279775143 | 10.876892090 | 0.000000000 |

## B. $H_2O$@*h*-BN (int)

Hartree-Fock energy: −1126.724 eV.

H2O@hBN (int)
1.0

| | | |
|---|---|---|
| 15.0714654922 | 0.0000000000 | 0.0000000000 |
| −7.5357344841 | 13.0522709851 | 0.0000000000 |
| 0.0000000000 | 0.0000000000 | 16.0000000000 |

| | | | |
|---|---|---|---|
| H | O | N | B |
| 2 | 1 | 36 | 36 |

Cartesian

| | | |
|---|---|---|
| 1.83595549 | 3.82563121 | 3.770000000 |
| 1.32595549 | 3.65563121 | 2.320000000 |
| 1.05595549 | 3.55563121 | 3.250000000 |
| 2.511910677 | 1.450252175 | 0.000000000 |
| 1.255954862 | 3.625631094 | 0.000000000 |
| −0.000000873 | 5.801009178 | 0.000000000 |
| −1.255956531 | 7.976387501 | 0.000000000 |
| −2.511912584 | 10.151766777 | 0.000000000 |
| −3.767868042 | 12.327144623 | 0.000000000 |

| | | |
|---|---|---|
| 5.023821831 | 1.450252175 | 0.000000000 |
| 3.767865658 | 3.625631094 | 0.000000000 |
| 2.511909962 | 5.801009178 | 0.000000000 |
| 1.255954385 | 7.976387501 | 0.000000000 |
| −0.000001583 | 10.151766777 | 0.000000000 |
| −1.255957007 | 12.327144623 | 0.000000000 |
| 7.535732746 | 1.450252175 | 0.000000000 |
| 6.279776573 | 3.625631094 | 0.000000000 |
| 5.023820877 | 5.801009178 | 0.000000000 |
| 3.767865181 | 7.976387501 | 0.000000000 |
| 2.511909246 | 10.151766777 | 0.000000000 |
| 1.255953908 | 12.327144623 | 0.000000000 |
| 10.047642708 | 1.450252175 | 0.000000000 |
| 8.791687012 | 3.625631094 | 0.000000000 |
| 7.535731316 | 5.801009178 | 0.000000000 |
| 6.279775620 | 7.976387501 | 0.000000000 |
| 5.023819923 | 10.151766777 | 0.000000000 |
| 3.767864227 | 12.327144623 | 0.000000000 |
| 12.559554100 | 1.450252175 | 0.000000000 |
| 11.303598404 | 3.625631094 | 0.000000000 |
| 10.047642708 | 5.801009178 | 0.000000000 |
| 8.791687012 | 7.976387501 | 0.000000000 |
| 7.535731316 | 10.151766777 | 0.000000000 |
| 6.279775620 | 12.327144623 | 0.000000000 |
| 0.000000255 | 1.450252175 | 0.000000000 |
| −1.255955696 | 3.625631094 | 0.000000000 |
| −2.511911392 | 5.801009178 | 0.000000000 |
| −3.767867088 | 7.976387501 | 0.000000000 |
| −5.023822784 | 10.151766777 | 0.000000000 |
| −6.279778481 | 12.327144623 | 0.000000000 |
| 0.000000000 | 0.000000000 | 0.000000000 |
| −1.255955815 | 2.175378561 | 0.000000000 |
| −2.511911631 | 4.350757122 | 0.000000000 |
| −3.767867327 | 6.526135445 | 0.000000000 |
| −5.023823261 | 8.701514244 | 0.000000000 |
| −6.279778957 | 10.876892090 | 0.000000000 |
| 2.511910915 | 0.000000000 | 0.000000000 |
| 1.255955100 | 2.175378561 | 0.000000000 |
| −0.000000711 | 4.350757122 | 0.000000000 |
| −1.255956411 | 6.526135445 | 0.000000000 |
| −2.511912346 | 8.701514244 | 0.000000000 |
| −3.767867804 | 10.876892090 | 0.000000000 |
| 5.023821831 | 0.000000000 | 0.000000000 |
| 3.767866135 | 2.175378561 | 0.000000000 |
| 2.511910200 | 4.350757122 | 0.000000000 |
| 1.255954504 | 6.526135445 | 0.000000000 |
| −0.000001421 | 8.701514244 | 0.000000000 |
| −1.255956888 | 10.876892090 | 0.000000000 |
| 7.535732746 | 0.000000000 | 0.000000000 |
| 6.279777050 | 2.175378561 | 0.000000000 |
| 5.023821354 | 4.350757122 | 0.000000000 |
| 3.767865419 | 6.526135445 | 0.000000000 |
| 2.511909485 | 8.701514244 | 0.000000000 |
| 1.255954027 | 10.876892090 | 0.000000000 |
| 10.047643661 | 0.000000000 | 0.000000000 |
| 8.791687965 | 2.175378561 | 0.000000000 |
| 7.535732269 | 4.350757122 | 0.000000000 |
| 6.279776573 | 6.526135445 | 0.000000000 |

```
   5.023820400       8.701514244      0.000000000
   3.767864943      10.876892090      0.000000000
  12.559554100       0.000000000      0.000000000
  11.303598404       2.175378561      0.000000000
  10.047642708       4.350757122      0.000000000
   8.791687012       6.526135445      0.000000000
   7.535730839       8.701514244      0.000000000
   6.279775143      10.876892090      0.000000000
```

### C. $CH_4$ in chabazite crystal

Hartree-Fock energy: $-635.295$ eV.

```
CH4 in Chab
   1.00533845683946
     9.2855642803100000    -0.3177687551000000     0.0000000000000000
    -0.3177687551000000     9.2855642803100000     0.0000000000000000
    -0.6580574218020000    -0.6580574218020000     9.2442740038999993
   O   Al  Si  H   C
   24   1  11  5   1
Direct
  0.5061580821527728  0.1410049477596802  0.4964802629983697
  0.6752186801914598  0.2201812953753326  0.2936708378446866
  0.8113700098480076  0.4935473203640653  0.2378809144784037
  0.7602309763800112  0.7018486712946492  0.4342323822407770
  0.5446012364976179  0.7960728928185957  0.5643667886220379
  0.2617847219606004  0.7544803354998473  0.5291549711059024
  0.2703867146561840  0.5871837992292602  0.2828524141361045
  0.3781487285453621  0.6228764928957944  0.0362917986658473
  0.5054258057282301  0.4554254033527503  0.2236334073774399
  0.6830163894882607  0.3307063789922405  0.0112240800336577
  0.5314083286421014  0.2271294780976277  0.7748181940133581
  0.5480892046887693  0.5104443464937115  0.8447618616377437
  0.2634961547695629  0.4704832742049995  0.8016168829334340
  0.1969071126113057  0.4708898070328870  0.5194082030445490
  0.2812498948573692  0.2339331760591802  0.6244597183541041
  0.0269885190109352  0.6454753279333907  0.3849895907403265
  0.3961334146012195  0.7307548307637801  0.7863397443346433
  0.7762081138856505  0.3929728762138042  0.7633239538643100
  0.8560501357650722  0.4573237301954712  0.5115270576951911
  0.6871847908690583  0.9611499929263497  0.3898113602244266
  0.5184265633881350  0.7399248463589118  0.2763469996057323
  0.0296467003200612  0.3230263937774085  0.6850636548148511
  0.7907494082378966  0.1848713071195958  0.5569195095424087
  0.3776617982815407  0.9852717047424097  0.6860315813244051
  0.6508882349629508  0.3589830901862447  0.1882061361150805
  0.6638876661381997  0.1294978461552984  0.4309965038137910
  0.8661813997407963  0.5792496303256630  0.4006235479056421
  0.6244976768075883  0.8006900762129899  0.4150238646845605
  0.3958095217894415  0.8171513018665824  0.6420874928977126
  0.1932419824365612  0.6138127245037114  0.4304308777986882
  0.4210280581573924  0.5971255714625467  0.2040409667559891
  0.4251780045904458  0.1474412473947995  0.6451178769792573
  0.6335674321452381  0.3632051474373815  0.8508247554222113
  0.3973374926361037  0.5828000995138817  0.8678574138035934
  0.1943861790658846  0.3747587432375889  0.6582402100444554
  0.8633160227096756  0.3370345317168018  0.6299739131955424
```

```
   0.8630418291501164   0.5216029286982651   0.1548396900152862
   0.0232579392426618   0.6922275825618235   0.8967243594837085
   0.0175774770087269   0.7067742400116142   0.0871906238289764
   0.9883454862293168   0.5339444874422024   0.9859359549855250
   0.8546463067912828   0.6645852864987718   0.9717474974724643
   0.9699710620002729   0.6490202557962372   0.9872509517970919
```

### D. $H_2O@TiO_2$ (far)

Hartree-Fock energy: −2939.878 eV.

```
H2O@TiO2 (far)
   1.00000000000000
    11.8360004424999996    0.0000000000000000    0.0000000000000000
     0.0000000000000000   12.9938001632999995    0.0000000000000000
     0.0000000000000000    0.0000000000000000   23.0000000000000000
   Ti   O   H
   48   97   2
Direct
   0.7506957176857725   0.7429537528022436   0.3746017513140600
   0.0006489231976090   0.7422232797837793   0.3684302951834795
   0.2506808985387252   0.7429585579793638   0.3690152835969371
   0.7491628746569674   0.2429612434482848   0.3673388748147985
   0.9989633888972804   0.2422443536836454   0.3758667088216114
   0.2491586726209718   0.2429877628109409   0.3758877124697975
   0.7497494383432084   0.4958314466083493   0.5084587614888676
   0.9997948647878161   0.5078660696868482   0.5081986574709845
   0.2496681070024280   0.4961178107348587   0.5086866959655083
   0.7498381781835874   0.9960429174762098   0.5083987478771945
   0.9999064536903361   0.0077521333262780   0.5083236327287111
   0.2500205108565510   0.9957872327981505   0.5087641803843894
   0.8748293901915218   0.4916693897204709   0.3712982229033557
   0.1247782130815622   0.4916261582680690   0.3714695784145334
   0.3748100372501213   0.4916963133827821   0.3720911291953826
   0.8748751814138203   0.9917925399290723   0.3713557929931000
   0.1248296397615860   0.9919512797467220   0.3716951260072250
   0.3748721286907326   0.9917728205563421   0.3720446096881673
   0.8707968395024537   0.7518252766556373   0.5218213706219288
   0.1159303400074521   0.7522447440848836   0.5192577712402340
   0.3619304848686795   0.7520029299404598   0.5216363674569848
   0.8752838312022959   0.2522012604253305   0.5226475181002925
   0.1311484183719998   0.2519323776220972   0.5236084905578196
   0.3875766473954059   0.2521496496156672   0.5223334936486026
   0.5006644137722347   0.7422192523348983   0.3750722068278165
   0.4989559323507962   0.2422609312533481   0.3674124596644432
   0.4997658707173755   0.5076593354937060   0.5087900105747138
   0.4996753263438336   0.0081759406960842   0.5086851398828927
   0.6247551753893390   0.4916220915607497   0.3719096348877002
   0.6248205770781112   0.9919208813507296   0.3717393344981659
   0.6168865437281141   0.7522483659851602   0.5229929949710268
   0.6314413553381613   0.2518582377241643   0.5183555804146280
   0.7496473626579672   0.4959850886073056   0.2347046029126858
   0.9997577102797734   0.5075396631111389   0.2345812735057251
   0.2497268401598873   0.4956897810443408   0.2348896654353112
   0.7499847826838888   0.9956570946097045   0.2346339821729515
   0.9996475471764370   0.0080853084720047   0.2347067566821721
   0.2497924701575940   0.9959404682230897   0.2349879251101186
```

| | | |
|---|---|---|
| 0.8617415139424409 | 0.7518970408651384 | 0.2219913167869123 |
| 0.1166603181015091 | 0.7521651329488535 | 0.2204667388675645 |
| 0.3704794999974297 | 0.7517198584769673 | 0.2217978612239619 |
| 0.8875264442203417 | 0.2520162796820600 | 0.2210139398487101 |
| 0.1314342541071127 | 0.2517645786760951 | 0.2247318908187168 |
| 0.3752917789957735 | 0.2521235547495664 | 0.2206682577985504 |
| 0.4997779089885768 | 0.5077606304796021 | 0.2351543029246699 |
| 0.4998687241261095 | 0.0076442098513922 | 0.2350537037304150 |
| 0.6157073933773134 | 0.7521653299122093 | 0.2241725538970627 |
| 0.6311087458819955 | 0.2518176734921980 | 0.2195709242073320 |
| 0.7496063750393986 | 0.4992701682147782 | 0.3151668745456391 |
| 0.9999536031822345 | 0.5019122117981496 | 0.3149606498619377 |
| 0.2502065166733587 | 0.4993285128641105 | 0.3152889138805790 |
| 0.7499370094433218 | 0.9993876920286624 | 0.3150665628618938 |
| 0.0002166773447243 | 0.0021642041143650 | 0.3150414214796555 |
| 0.2502760123813843 | 0.9994885545949899 | 0.3153897590321861 |
| 0.7552146359169356 | 0.7536051479203394 | 0.4553079155480049 |
| 0.0041186019168720 | 0.7505116199957129 | 0.4577862810111384 |
| 0.2539194014458630 | 0.7540345791952845 | 0.4579952982117774 |
| 0.7467065257709962 | 0.2538894454939040 | 0.4584038946260662 |
| 0.9961872421724749 | 0.2502006991750818 | 0.4552311229020205 |
| 0.2443368046873786 | 0.2536253437707785 | 0.4554857356380921 |
| 0.7480169540440826 | 0.7525293129542163 | 0.5682305928064082 |
| 0.9974788821530467 | 0.7508847743567841 | 0.5690921484056233 |
| 0.2467594019285073 | 0.7524589361499849 | 0.5697175699917523 |
| 0.7513737103088260 | 0.2524329427008638 | 0.5694896473658204 |
| 0.0011082021302542 | 0.2507049163948096 | 0.5682831076136168 |
| 0.2513433028142700 | 0.2525491542321916 | 0.5687897354379032 |
| 0.7502305172818637 | 0.4993895904626910 | 0.4280568261842888 |
| 0.9997184831451591 | 0.5019454009882836 | 0.4278887971673129 |
| 0.2496104625242452 | 0.4992777087405997 | 0.4282046092714253 |
| 0.7503197358312121 | 0.9996025820349459 | 0.4279987763524389 |
| 0.9997850049636767 | 0.0022264790588622 | 0.4280066654114307 |
| 0.2499800209304439 | 0.9995485535627111 | 0.4283295593351042 |
| 0.8783103387195723 | 0.8526740632774050 | 0.3713722358206510 |
| 0.1258536281386569 | 0.8527701005928989 | 0.3722992842994728 |
| 0.3782840153025973 | 0.8526672692638115 | 0.3721352973842045 |
| 0.8747176417028797 | 0.3524128695967761 | 0.3711958470748087 |
| 0.1222415189077495 | 0.3525849612691019 | 0.3708106356783887 |
| 0.3747312359599491 | 0.3524218800267107 | 0.3721148363406641 |
| 0.8727025347234729 | 0.5947687663299916 | 0.5219084582775650 |
| 0.1259312639562040 | 0.5946234202867799 | 0.5228564455439511 |
| 0.3737284987688696 | 0.5949414203720949 | 0.5218963296301027 |
| 0.8741060119460897 | 0.0948876968241592 | 0.5218687502039785 |
| 0.1263404174614706 | 0.0950318801177872 | 0.5209185509876093 |
| 0.3729448330046665 | 0.0947946707438803 | 0.5224727596251881 |
| 0.8759260723418691 | 0.6491680694349711 | 0.3712379508088404 |
| 0.1275854836898347 | 0.6491676311006103 | 0.3721212260834434 |
| 0.3758928024508705 | 0.6491533918540142 | 0.3722494591421821 |
| 0.8727748729574856 | 0.1492972825157395 | 0.3710440911995221 |
| 0.1245354978019435 | 0.1493005962670821 | 0.3710702575142122 |
| 0.3727847460077243 | 0.1493127158875041 | 0.3721866546345609 |
| 0.8756221120769325 | 0.9091027297486960 | 0.5226239933260004 |
| 0.1231708855596949 | 0.9093835263395107 | 0.5235257874972135 |
| 0.3768040251207125 | 0.9091888665077548 | 0.5229098127171241 |
| 0.8769771944979681 | 0.4092047319107124 | 0.5226147605587528 |
| 0.1232864143171355 | 0.4088656538785642 | 0.5215520912058054 |
| 0.3756117749032910 | 0.4091484833280532 | 0.5229128688080351 |

| | | |
|---|---|---|
| 0.4997129214777800 | 0.5019518606668072 | 0.3154526441073315 |
| 0.4998147912872142 | 0.0020493401735067 | 0.3153729650518784 |
| 0.5061387563023203 | 0.7504841410835752 | 0.4555893613891939 |
| 0.4974223135849982 | 0.2504442901933501 | 0.4591682927883980 |
| 0.4977360725077702 | 0.7506488372346922 | 0.5686697996980712 |
| 0.5027123548696650 | 0.2508672361205484 | 0.5703776930604647 |
| 0.4999506082348049 | 0.5019057619797778 | 0.4283846017479647 |
| 0.5001881570255051 | 0.0022181645184958 | 0.4283353888861114 |
| 0.6258833318848005 | 0.8527463227029770 | 0.3712396190774783 |
| 0.6223149167671806 | 0.3525854744955979 | 0.3724483955776208 |
| 0.6262327059426553 | 0.5950038386060683 | 0.5211101116774159 |
| 0.6267478764173973 | 0.0945971210358110 | 0.5230385221537617 |
| 0.6275980874264278 | 0.6491639856454512 | 0.3713349568304878 |
| 0.6245365595728245 | 0.1492877109632360 | 0.3721779159071303 |
| 0.6234190921674738 | 0.9089414559478897 | 0.5217213498938165 |
| 0.6237009705264711 | 0.4093007092675904 | 0.5236895604683625 |
| 0.7466745508961878 | 0.7523614425904412 | 0.1738118594938669 |
| 0.9975997840691520 | 0.7504587734587673 | 0.1747963628306053 |
| 0.2478970070661290 | 0.7524428524257871 | 0.1752582910620930 |
| 0.7513326251585966 | 0.2524481525618967 | 0.1743965432372008 |
| 0.0025652669606160 | 0.2507011517599480 | 0.1728400146123548 |
| 0.2514685240711003 | 0.2523046909049356 | 0.1737032070870157 |
| 0.7539610541763864 | 0.7540186643830395 | 0.2855082367350121 |
| 0.0061061532010172 | 0.7504408927301611 | 0.2878917276120703 |
| 0.2553299249834708 | 0.7535964306483933 | 0.2882078607713723 |
| 0.7444042373625308 | 0.2536271560839722 | 0.2877121556187490 |
| 0.9974518032657684 | 0.2504085848204483 | 0.2840171583741764 |
| 0.2466201548111044 | 0.2539698772451189 | 0.2847710620514476 |
| 0.8736598317109312 | 0.5947976946475109 | 0.2214878117347183 |
| 0.1261909371035443 | 0.5949444664723345 | 0.2224032305833035 |
| 0.3726178962659006 | 0.5946368698114810 | 0.2215005206679095 |
| 0.8728229166810380 | 0.0946914327842663 | 0.2209490905834741 |
| 0.1267485802882220 | 0.0944557503584775 | 0.2201563586768458 |
| 0.3740484760832317 | 0.0948368713319141 | 0.2216551850617634 |
| 0.8768198121796260 | 0.9090824774880133 | 0.2205358823952892 |
| 0.1233208925170999 | 0.9088154054381548 | 0.2217861483018027 |
| 0.3755958328685267 | 0.9090180819402391 | 0.2207607325933125 |
| 0.8755802483452939 | 0.4090070637777856 | 0.2204191194047880 |
| 0.1236412529048394 | 0.4092832873912187 | 0.2193519741135077 |
| 0.3770134124404834 | 0.4090810722448879 | 0.2207143902938000 |
| 0.4972627840602044 | 0.7506779044993621 | 0.1744224151484985 |
| 0.5010517107990395 | 0.2504938834885735 | 0.1749132679608039 |
| 0.5041427555722535 | 0.7505005138772916 | 0.2857318921744181 |
| 0.4961941619914256 | 0.2502589374194102 | 0.2879974543828183 |
| 0.6259354662813124 | 0.5945055906954479 | 0.2205558830268544 |
| 0.6262967202936451 | 0.0949368026727129 | 0.2224098570363964 |
| 0.6230985144200289 | 0.9092900821511094 | 0.2198238655432689 |
| 0.6232580285812972 | 0.4087707153621878 | 0.2216400129064553 |
| 0.4951504905285518 | 0.5413441128537073 | 0.8716365217391271 |
| 0.4984750557979680 | 0.6180364795575315 | 0.8710702464782614 |
| 0.5547092058585008 | 0.5159859602071393 | 0.8966170253043444 |

## E. $H_2O$@$TiO_2$ (int, unrelaxed)

Hartree-Fock energy: −2940.622 eV.

H2O@TiOs (int unrelaxed)

```
   1.00000000000000
    11.8360004424999996     0.0000000000000000     0.0000000000000000
     0.0000000000000000    12.9938001632999995     0.0000000000000000
     0.0000000000000000     0.0000000000000000    23.0000000000000000
   Ti    O    H
   48   97    2
Direct
  0.7506957176857725  0.7429537528022436  0.3746017513140600
  0.0006489231976090  0.7422232797837793  0.3684302951834795
  0.2506808985387252  0.7429585579793638  0.3690152835969371
  0.7491628746569674  0.2429612434482848  0.3673388748147985
  0.9989633888972804  0.2422443536836454  0.3758667088216114
  0.2491586726209718  0.2429877628109409  0.3758877124697975
  0.7497494383432084  0.4958314466083493  0.5084587614888676
  0.9997948647878161  0.5078660696868482  0.5081986574709845
  0.2496681070024280  0.4961178107348587  0.5086866959655083
  0.7498381781835874  0.9960429174762098  0.5083987478771945
  0.9999064536903361  0.0077521333262780  0.5083236327287111
  0.2500205108565510  0.9957872327981505  0.5087641803843894
  0.8748293901915218  0.4916693897204709  0.3712982229033557
  0.1247782130815622  0.4916261582680690  0.3714695784145334
  0.3748100372501213  0.4916963133827821  0.3720911291953826
  0.8748751814138203  0.9917925399290723  0.3713557929931000
  0.1248296397615860  0.9919512797467220  0.3716951260072250
  0.3748721286907326  0.9917728205563421  0.3720446096881673
  0.8707968395024537  0.7518252766556373  0.5218213706219288
  0.1159303400074521  0.7522447440848836  0.5192577712402340
  0.3619304848686795  0.7520029299404598  0.5216363674569848
  0.8752838312022959  0.2522012604253305  0.5226475181002925
  0.1311484183719998  0.2519323776220972  0.5236084905578196
  0.3875766473954059  0.2521496496156672  0.5223334936486026
  0.5006644137722347  0.7422192523348983  0.3750722068278165
  0.4989559323507962  0.2422609312533481  0.3674124596644432
  0.4997658707173755  0.5076593354937060  0.5087900105747138
  0.4996753263438336  0.0081759406960842  0.5086851398828927
  0.6247551753893390  0.4916220915607497  0.3719096348877002
  0.6248205770781112  0.9919208813507296  0.3717393344981659
  0.6168865437281141  0.7522483659851602  0.5229929949710268
  0.6314413553381613  0.2518582377241643  0.5183555804146280
  0.7496473626579672  0.4959850886073056  0.2347046029126858
  0.9997577102797734  0.5075396631111389  0.2345812735057251
  0.2497268401598873  0.4956897810443408  0.2348896654353112
  0.7499847826838888  0.9956570946097045  0.2346339821729515
  0.9996475471764370  0.0080853084720047  0.2347067566821721
  0.2497924701575940  0.9959404682230897  0.2349879251101186
  0.8617415139424409  0.7518970408651384  0.2219913167869123
  0.1166603181015091  0.7521651329488535  0.2204667388675645
  0.3704794999974297  0.7517198584769673  0.2217978612239619
  0.8875264442203417  0.2520162796820600  0.2210139398487101
  0.1314342541071127  0.2517645786760951  0.2247318908187168
  0.3752917789957735  0.2521235547495664  0.2206682577985504
  0.4997779089885768  0.5077606304796021  0.2351543029246699
  0.4998687241261095  0.0076442098513922  0.2350537037304150
  0.6157073933773134  0.7521653299122093  0.2241725538970627
  0.6311087458819955  0.2518176734921980  0.2195709242073320
  0.7496063750393986  0.4992701682147782  0.3151668745456391
  0.9999536031822345  0.5019122117981496  0.3149606498619377
  0.2502065166733587  0.4993285128641105  0.3152889138805790
```

| | | |
|---|---|---|
| 0.7499370094433218 | 0.9993876920286624 | 0.3150665628618938 |
| 0.0002166773447243 | 0.0021642041143650 | 0.3150414214796555 |
| 0.2502760123813843 | 0.9994885545949899 | 0.3153897590321861 |
| 0.7552146359169356 | 0.7536051479203394 | 0.4553079155480049 |
| 0.0041186019168720 | 0.7505116199957129 | 0.4577862810111384 |
| 0.2539194014458630 | 0.7540345791952845 | 0.4579952982117774 |
| 0.7467065257709962 | 0.2538894454939040 | 0.4584038946260662 |
| 0.9961872421724749 | 0.2502006991750818 | 0.4552311229020205 |
| 0.2443368046873786 | 0.2536253437707785 | 0.4554857356380921 |
| 0.7480169540440826 | 0.7525293129542163 | 0.5682305928064082 |
| 0.9974788821530467 | 0.7508847743567841 | 0.5690921484056233 |
| 0.2467594019285073 | 0.7524589361499849 | 0.5697175699917523 |
| 0.7513737103088260 | 0.2524329427008638 | 0.5694896473658204 |
| 0.0011082021302542 | 0.2507049163948096 | 0.5682831076136168 |
| 0.2513433028142700 | 0.2525491542321916 | 0.5687897354379032 |
| 0.7502305172818637 | 0.4993895904626910 | 0.4280568261842888 |
| 0.9997184831451591 | 0.5019454009882836 | 0.4278887971673129 |
| 0.2496104625242452 | 0.4992777087405997 | 0.4282046092714253 |
| 0.7503197358312121 | 0.9996025820349459 | 0.4279987763524389 |
| 0.9997850049636767 | 0.0022264790588622 | 0.4280066654114307 |
| 0.2499800209304439 | 0.9995485535627111 | 0.4283295593351042 |
| 0.8783103387195723 | 0.8526740632774050 | 0.3713722358206510 |
| 0.1258536281386569 | 0.8527701005928989 | 0.3722992842994728 |
| 0.3782840153025973 | 0.8526672692638115 | 0.3721352973842045 |
| 0.8747176417028797 | 0.3524128695967761 | 0.3711958470748087 |
| 0.1222415189077495 | 0.3525849612691019 | 0.3708106356783887 |
| 0.3747312359599491 | 0.3524218800267107 | 0.3721148363406641 |
| 0.8727025347234729 | 0.5947687663299916 | 0.5219084582775650 |
| 0.1259312639562040 | 0.5946234202867799 | 0.5228564455439511 |
| 0.3737284987688696 | 0.5949414203720949 | 0.5218963296301027 |
| 0.8741060119460897 | 0.0948876968241592 | 0.5218687502039785 |
| 0.1263404174614706 | 0.0950318801177872 | 0.5209185509876093 |
| 0.3729448330046665 | 0.0947946707438803 | 0.5224727596251881 |
| 0.8759260723418691 | 0.6491680694349711 | 0.3712379508088404 |
| 0.1275854836898347 | 0.6491676311006103 | 0.3721212260834434 |
| 0.3758928024508705 | 0.6491533918540142 | 0.3722494591421821 |
| 0.8727748729574856 | 0.1492972825157395 | 0.3710440911995221 |
| 0.1245354978019435 | 0.1493005962670821 | 0.3710702575142122 |
| 0.3727847460077243 | 0.1493127158875041 | 0.3721866546345609 |
| 0.8756221120769325 | 0.9091027297486960 | 0.5226239933260004 |
| 0.1231708855596949 | 0.9093835263395107 | 0.5235257874972135 |
| 0.3768040251207125 | 0.9091888665077548 | 0.5229098127171241 |
| 0.8769771944979681 | 0.4092047319107124 | 0.5226147605587528 |
| 0.1232864143171355 | 0.4088656538785642 | 0.5215520912058054 |
| 0.3756117749032910 | 0.4091484833280532 | 0.5229128688080351 |
| 0.4997129214777800 | 0.5019518606668072 | 0.3154526441073315 |
| 0.4998147912872142 | 0.0020493401735067 | 0.3153729650518784 |
| 0.5061387563023203 | 0.7504841410835752 | 0.4555893613891939 |
| 0.4974223135849982 | 0.2504442901933501 | 0.4591682927883980 |
| 0.4977360725077702 | 0.7506488372346922 | 0.5686697996980712 |
| 0.5027123548696650 | 0.2508672361205484 | 0.5703776930604647 |
| 0.4999506082348049 | 0.5019057619797778 | 0.4283846017479647 |
| 0.5001881570255051 | 0.0022181645184958 | 0.4283353888861114 |
| 0.6258833318848005 | 0.8527463227029770 | 0.3712396190774783 |
| 0.6223149167671806 | 0.3525854744955979 | 0.3724483955776208 |
| 0.6262327059426553 | 0.5950038386060683 | 0.5211101116774159 |
| 0.6267478764173973 | 0.0945971210358110 | 0.5230385221537617 |
| 0.6275980874264278 | 0.6491639856454512 | 0.3713349568304878 |

```
  0.6245365595728245  0.1492877109632360  0.3721779159071303
  0.6234190921674738  0.9089414559478897  0.5217213498938165
  0.6237009705264711  0.4093007092675904  0.5236895604683625
  0.7466745508961878  0.7523614425904412  0.1738118594938669
  0.9975997840691520  0.7504587734587673  0.1747963628306053
  0.2478970070661290  0.7524428524257871  0.1752582910620930
  0.7513326251585966  0.2524481525618967  0.1743965432372008
  0.0025652669606160  0.2507011517599480  0.1728400146123548
  0.2514685240711003  0.2523046909049356  0.1737032070870157
  0.7539610541763864  0.7540186643830395  0.2855082367350121
  0.0061061532010172  0.7504408927301611  0.2878917276120703
  0.2553299249834708  0.7535964306483933  0.2882078607713723
  0.7444042373625308  0.2536271560839722  0.2877121556187490
  0.9974518032657684  0.2504085848204483  0.2840171583741764
  0.2466201548111044  0.2539698772451189  0.2847710620514476
  0.8736598317109312  0.5947976946475109  0.2214878117347183
  0.1261909371035443  0.5949444664723345  0.2224032305833035
  0.3726178962659006  0.5946368698114810  0.2215005206679095
  0.8728229166810380  0.0946914327842663  0.2209490905834741
  0.1267485802882220  0.0944557503584775  0.2201563586768458
  0.3740484760832317  0.0948368713319141  0.2216551850617634
  0.8768198121796260  0.9090824774880133  0.2205358823952892
  0.1233208925170999  0.9088154054381548  0.2217861483018027
  0.3755958328685267  0.9090180819402391  0.2207607325933125
  0.8755802483452939  0.4090070637777856  0.2204191194047880
  0.1236412529048394  0.4092832873912187  0.2193519741135077
  0.3770134124404834  0.4090810722448879  0.2207143902938000
  0.4972627840602044  0.7506779044993621  0.1744224151484985
  0.5010517107990395  0.2504938834885735  0.1749132679608039
  0.5041427555722535  0.7505005138772916  0.2857318921744181
  0.4961941619914256  0.2502589374194102  0.2879974543828183
  0.6259354662813124  0.5945055906954479  0.2205558830268544
  0.6262967202936451  0.0949368026727129  0.2224098570363964
  0.6230985144200289  0.9092900821511094  0.2198238655432689
  0.6232580285812972  0.4087707153621878  0.2216400129064553
  0.4951504905285518  0.5413441128537073  0.6046243336086974
  0.4984750557979680  0.6180364795575315  0.6040580583478246
  0.5547092058585008  0.5159859602071393  0.6296048371739147
```

### F. $H_2O@TiO_2$ (int, relaxed using DFT-PBE)

Hartree-Fock energy: −2940.857 eV.

```
H2O@TiOs (int relaxed)
   1.00000000000000
     11.8360004424999996     0.0000000000000000     0.0000000000000000
      0.0000000000000000    12.9938001632999995     0.0000000000000000
      0.0000000000000000     0.0000000000000000    23.0000000000000000
   Ti    O    H
   48    97    2
Direct
  0.7513669333760750  0.7430476126832284  0.3748697021293116
  0.0011521538136454  0.7422546475672563  0.3653417054870843
  0.2509456697123438  0.7428316794528217  0.3657732038250702
  0.7493450184340675  0.2429354307598557  0.3646387882206389
  0.9991097641861252  0.2420384877861418  0.3766097360477613
  0.2499284731775843  0.2428171641398907  0.3767273050211717
```

| | | |
|---|---|---|
| 0.7501621141945434 | 0.5061820363111261 | 0.5058448576873553 |
| 0.9998410879242035 | 0.4972109285123157 | 0.5058986856008467 |
| 0.2489855777603444 | 0.5060117191706773 | 0.5065077868224027 |
| 0.7505491038232553 | 0.9980687238866374 | 0.5082693881596106 |
| 0.0003582753942973 | 0.0053542306197116 | 0.5082171177392639 |
| 0.2501326882477353 | 0.9971743199258768 | 0.5087046194847255 |
| 0.8746419421497348 | 0.4911373098786414 | 0.3685340960290931 |
| 0.1255044543413422 | 0.4909278736142297 | 0.3688508888163854 |
| 0.3775865949136969 | 0.4917950243063932 | 0.3737926869962929 |
| 0.8751600329110106 | 0.9919091889955913 | 0.3709096578091450 |
| 0.1251519811805395 | 0.9922366054721465 | 0.3713227708790806 |
| 0.3752178419871266 | 0.9920040315320244 | 0.3715792938758824 |
| 0.8765661319984256 | 0.7515770733779700 | 0.5214862895092587 |
| 0.1179331061110680 | 0.7515153063994123 | 0.5180219442843041 |
| 0.3616706963318111 | 0.7527132884200840 | 0.5197832423143383 |
| 0.8717645117700730 | 0.2526675788201939 | 0.5234659678434909 |
| 0.1299657791974325 | 0.2522142630184684 | 0.5240464296410497 |
| 0.3873715722780443 | 0.2509174228812850 | 0.5232957047905686 |
| 0.5010603613614044 | 0.7430216643966371 | 0.3755756842519044 |
| 0.4993351474714515 | 0.2429627039298391 | 0.3653347071265274 |
| 0.4986939949353230 | 0.4971281547087708 | 0.5152677254363323 |
| 0.5003082212890972 | 0.0054717587099804 | 0.5085787349539059 |
| 0.6226046909625270 | 0.4916322625336109 | 0.3733289391625580 |
| 0.6251500263902937 | 0.9923250617806879 | 0.3712236509250896 |
| 0.6204225782494427 | 0.7521936820270372 | 0.5220523472162888 |
| 0.6304215741816397 | 0.2514826782332302 | 0.5168994049993200 |
| 0.7494846156837945 | 0.4965379720455007 | 0.2338397090606833 |
| −0.0000037539801940 | 0.5054855257585862 | 0.2324013800043599 |
| 0.2503932282183477 | 0.4961057301608630 | 0.2342070853777300 |
| 0.7501845923323935 | 0.9950675552689012 | 0.2341812542553981 |
| 0.9998782976775766 | 0.0070860537223981 | 0.2342701119509701 |
| 0.2499388841854294 | 0.9955897887584122 | 0.2346156379755295 |
| 0.8627972409190452 | 0.7508969887268746 | 0.2195376779323223 |
| 0.1198267215548327 | 0.7510952688918712 | 0.2179420380841721 |
| 0.3759414842241690 | 0.7506412350806689 | 0.2194809519022929 |
| 0.8861219749328701 | 0.2509717280364683 | 0.2183311227310341 |
| 0.1281085235787294 | 0.2509358046211064 | 0.2250435785125686 |
| 0.3701036679582194 | 0.2509974890318131 | 0.2187661032908212 |
| 0.4998790783289109 | 0.5053024938692000 | 0.2350032795556645 |
| 0.5000804453317541 | 0.0064688848868343 | 0.2346058537710043 |
| 0.6190636161186586 | 0.7508289831299678 | 0.2244513185367150 |
| 0.6279949422676834 | 0.2508892376518208 | 0.2175507510698698 |
| 0.7489982245672068 | 0.4996847904212410 | 0.3138072853447628 |
| 0.0003311058136390 | 0.5016772579550836 | 0.3128553585685928 |
| 0.2515235008683927 | 0.4995840761406655 | 0.3141427809818529 |
| 0.7504170583360762 | 0.9999061506545210 | 0.3146596721606325 |
| 0.0004222184473844 | 0.0023117816522331 | 0.3147142315248315 |
| 0.2504350571931570 | −0.0000169214015301 | 0.3150823030196099 |
| 0.7544911776890818 | 0.7555705693828283 | 0.4542020813738727 |
| 0.0027499673478168 | 0.7518930414429008 | 0.4587822279153326 |
| 0.2518994878235192 | 0.7560335718501756 | 0.4583647551927203 |
| 0.7475397108570941 | 0.2530255811992240 | 0.4596613006763057 |
| 0.9984878879883419 | 0.2504718121102119 | 0.4547676588202483 |
| 0.2452546244781323 | 0.2515496075229701 | 0.4552344277595297 |
| 0.7482588345662058 | 0.7491971121333771 | 0.5671251422431819 |
| 0.9986164719110091 | 0.7510897046697980 | 0.5694523623787272 |
| 0.2490219695672756 | 0.7496322966990024 | 0.5693185288070548 |
| 0.7511385608342140 | 0.2516541689011425 | 0.5704193083061344 |

| | | |
|---|---|---|
| 0.0013978764104219 | 0.2506197825708568 | 0.5682503719396379 |
| 0.2512930754601659 | 0.2520283012862314 | 0.5690081162773412 |
| 0.7524175625671833 | 0.4985870467705938 | 0.4259018569856336 |
| 0.9998503962541883 | 0.4994276198344472 | 0.4257276335612981 |
| 0.2480069191651799 | 0.4995355026811830 | 0.4264375453679079 |
| 0.7504557920924884 | 0.9988309510668091 | 0.4279301309040374 |
| 0.0000673974999533 | 0.0005563745805282 | 0.4279852450087799 |
| 0.2504516660926654 | 0.9988096949110875 | 0.4283477955569809 |
| 0.8780332206204395 | 0.8524318401101642 | 0.3699298991077684 |
| 0.1256645921495714 | 0.8524783034093570 | 0.3711851177387898 |
| 0.3770249555667490 | 0.8525160030819755 | 0.3705062330300584 |
| 0.8753280975275569 | 0.3512688041405275 | 0.3693262892969609 |
| 0.1235737602412322 | 0.3515754202381765 | 0.3691488782249348 |
| 0.3744068904652752 | 0.3513462269302047 | 0.3715126994649528 |
| 0.8748690396213543 | 0.5946584825069750 | 0.5204335905153978 |
| 0.1244971904195649 | 0.5944969169448885 | 0.5215285410778415 |
| 0.3722826078380581 | 0.5965968590482711 | 0.5149638489521652 |
| 0.8751522326811564 | 0.0945467805745190 | 0.5213903456199765 |
| 0.1265993460612660 | 0.0944859081502015 | 0.5205290039072096 |
| 0.3740406491317331 | 0.0942798263477175 | 0.5224754449886051 |
| 0.8761559003311105 | 0.6491474006971133 | 0.3703436756515341 |
| 0.1268861843054861 | 0.6493030118440819 | 0.3714656882794976 |
| 0.3760499253254178 | 0.6493388900001351 | 0.3724456528207480 |
| 0.8736692861095710 | 0.1487378045773469 | 0.3709676774850170 |
| 0.1249021871664982 | 0.1485714929945749 | 0.3706204180011463 |
| 0.3740854827488383 | 0.1489001808832044 | 0.3720150024174013 |
| 0.8750230680044796 | 0.9088639303651931 | 0.5232877514731569 |
| 0.1243611643586143 | 0.9090078043680755 | 0.5243504786250714 |
| 0.3777854815914884 | 0.9086071572971764 | 0.5242845544819071 |
| 0.8774261692498960 | 0.4083763175899167 | 0.5212704265962070 |
| 0.1243442942321358 | 0.4081614149083153 | 0.5200201184925167 |
| 0.3730585622424208 | 0.4090407529586895 | 0.5216524469073078 |
| 0.4997754840786220 | 0.5015768718674188 | 0.3154169766960208 |
| 0.4999597800177826 | 0.0022396774742095 | 0.3150306025376405 |
| 0.5048111256800906 | 0.7566080472576401 | 0.4548215067643468 |
| 0.4999047027135690 | 0.2511283608226231 | 0.4603934698669064 |
| 0.5002285137397026 | 0.7389462318282245 | 0.5689150528084731 |
| 0.5020485318451766 | 0.2529765292867969 | 0.5712492847518588 |
| 0.5005384919404063 | 0.4976210339224964 | 0.4286531692400450 |
| 0.5005145619761867 | 0.0003991161707045 | 0.4282637334356385 |
| 0.6262213324012550 | 0.8527552851263224 | 0.3693822790244294 |
| 0.6244966233083186 | 0.3514761302636730 | 0.3717102894159103 |
| 0.6299286916073256 | 0.5976805132009914 | 0.5124912638745681 |
| 0.6264724249288420 | 0.0944245433925557 | 0.5233713847137342 |
| 0.6269418291810892 | 0.6493261484137355 | 0.3715186953215925 |
| 0.6249416823175664 | 0.1488652777921296 | 0.3720557432469722 |
| 0.6241169494013203 | 0.9084802760698713 | 0.5227783907357516 |
| 0.6272081031076090 | 0.4108741804299720 | 0.5254770025090504 |
| 0.7472554725159685 | 0.7520272780032700 | 0.1718313524999021 |
| 0.9987567410241045 | 0.7506117185453536 | 0.1731089171096459 |
| 0.2493048253461605 | 0.7521777823682326 | 0.1736357462679690 |
| 0.7503244630157896 | 0.2513447016079700 | 0.1728780336769999 |
| 0.0019737160341472 | 0.2498218772287815 | 0.1708357512839608 |
| 0.2504237286140814 | 0.2512200741553602 | 0.1718388213362727 |
| 0.7523129231358007 | 0.7518564044896180 | 0.2830411694682626 |
| 0.0052035508502918 | 0.7492495564020070 | 0.2864397486589827 |
| 0.2531798948052961 | 0.7511211719846617 | 0.2868236861323261 |
| 0.7460349199764934 | 0.2508806173695991 | 0.2864456545412806 |

```
0.9994475519558437   0.2490365321091974   0.2816111851380027
0.2479218269148800   0.2515745161010458   0.2826083316126069
0.8744077720562556   0.5938773235186848   0.2192240082049914
0.1262380558203810   0.5940836604057954   0.2206344146924547
0.3734787647730383   0.5936832345281027   0.2201701572013223
0.8729687197545669   0.0934926020362379   0.2196849799250809
0.1266056061369719   0.0931916476885571   0.2187813669781490
0.3745948421570140   0.0936777548204410   0.2206557307485446
0.8770644220060304   0.9080341704006324   0.2203147246481909
0.1238460770263261   0.9076389420398726   0.2220178918016812
0.3753307612564918   0.9078893898991353   0.2207759945297786
0.8750844921600368   0.4078596966945898   0.2193089932590750
0.1242630963192961   0.4081628538710376   0.2182459085736213
0.3772670485988199   0.4079193455935092   0.2202541725954246
0.4990190071753946   0.7505678791573134   0.1727497673883380
0.5003835477909329   0.2495389831603647   0.1735944881922259
0.5029610965728011   0.7496871567965813   0.2837803338681497
0.4991000159924912   0.2493667241520592   0.2871773448172246
0.6253150407665241   0.5934839191620614   0.2191047133593743
0.6261777531980189   0.0938779510294937   0.2217281561165175
0.6235543799585708   0.9082802624323012   0.2194625102136573
0.6234344035203442   0.4075563474511770   0.2214934709983579
0.4951504905285518   0.5413441128537073   0.6046243336086974
0.4984750557979680   0.6180364795575315   0.6040580583478246
0.5547092058585008   0.5159859602071393   0.6296048371739147
```

## G. NaCl pristine cell

Hartree-Fock energy: $-1375.880$ eV.

```
LiCl pristine
  1.00000000000000
   15.4731335457707697    0.0000000000000000    0.0000000000000000
    0.0000000000000000   15.4731335457707697    0.0000000000000000
    0.0000000000000000    0.0000000000000000   15.4731335457707697
  Cl   Li
  108  108
Direct
0.0000000000000000   0.0000000000000000   0.0000000000000000
0.0000000000000000   0.1666666666666643   0.1666666666666643
0.0000000000000000   0.3333333333333357   0.3333333333333357
0.0000000000000000   0.5000000000000000   0.5000000000000000
0.0000000000000000   0.6666666666666643   0.6666666666666643
0.0000000000000000   0.8333333333333357   0.8333333333333357
0.1666666666666643   0.0000000000000000   0.1666666666666643
0.1666666666666643   0.1666666666666643   0.3333333333333357
0.1666666666666643   0.3333333333333357   0.5000000000000000
0.1666666666666643   0.5000000000000000   0.6666666666666643
0.1666666666666643   0.6666666666666643   0.8333333333333357
0.1666666666666643   0.8333333333333357   0.0000000000000000
0.3333333333333357   0.0000000000000000   0.3333333333333357
0.3333333333333357   0.1666666666666643   0.5000000000000000
0.3333333333333357   0.3333333333333357   0.6666666666666643
0.3333333333333357   0.5000000000000000   0.8333333333333357
0.3333333333333357   0.6666666666666643   0.0000000000000000
0.3333333333333357   0.8333333333333357   0.1666666666666643
0.5000000000000000   0.0000000000000000   0.5000000000000000
```

| | | |
|---|---|---|
| 0.5000000000000000 | 0.1666666666666643 | 0.6666666666666643 |
| 0.5000000000000000 | 0.3333333333333357 | 0.8333333333333357 |
| 0.5000000000000000 | 0.5000000000000000 | 0.0000000000000000 |
| 0.5000000000000000 | 0.6666666666666643 | 0.1666666666666643 |
| 0.5000000000000000 | 0.8333333333333357 | 0.3333333333333357 |
| 0.6666666666666643 | 0.0000000000000000 | 0.6666666666666643 |
| 0.6666666666666643 | 0.1666666666666643 | 0.8333333333333357 |
| 0.6666666666666643 | 0.3333333333333357 | 0.0000000000000000 |
| 0.6666666666666643 | 0.5000000000000000 | 0.1666666666666643 |
| 0.6666666666666643 | 0.6666666666666643 | 0.3333333333333357 |
| 0.6666666666666643 | 0.8333333333333357 | 0.5000000000000000 |
| 0.8333333333333357 | 0.0000000000000000 | 0.8333333333333357 |
| 0.8333333333333357 | 0.1666666666666643 | 0.0000000000000000 |
| 0.8333333333333357 | 0.3333333333333357 | 0.1666666666666643 |
| 0.8333333333333357 | 0.5000000000000000 | 0.3333333333333357 |
| 0.8333333333333357 | 0.6666666666666643 | 0.5000000000000000 |
| 0.8333333333333357 | 0.8333333333333357 | 0.6666666666666643 |
| 0.1666666666666643 | 0.1666666666666643 | 0.0000000000000000 |
| 0.1666666666666643 | 0.3333333333333357 | 0.1666666666666643 |
| 0.1666666666666643 | 0.5000000000000000 | 0.3333333333333357 |
| 0.1666666666666643 | 0.6666666666666643 | 0.5000000000000000 |
| 0.1666666666666643 | 0.8333333333333357 | 0.6666666666666643 |
| 0.1666666666666643 | 0.0000000000000000 | 0.8333333333333357 |
| 0.3333333333333357 | 0.1666666666666643 | 0.1666666666666643 |
| 0.3333333333333357 | 0.3333333333333357 | 0.3333333333333357 |
| 0.3333333333333357 | 0.5000000000000000 | 0.5000000000000000 |
| 0.3333333333333357 | 0.6666666666666643 | 0.6666666666666643 |
| 0.3333333333333357 | 0.8333333333333357 | 0.8333333333333357 |
| 0.3333333333333357 | 0.0000000000000000 | 0.0000000000000000 |
| 0.5000000000000000 | 0.1666666666666643 | 0.3333333333333357 |
| 0.5000000000000000 | 0.3333333333333357 | 0.5000000000000000 |
| 0.5000000000000000 | 0.5000000000000000 | 0.6666666666666643 |
| 0.5000000000000000 | 0.6666666666666643 | 0.8333333333333357 |
| 0.5000000000000000 | 0.8333333333333357 | 0.0000000000000000 |
| 0.5000000000000000 | 0.0000000000000000 | 0.1666666666666643 |
| 0.6666666666666643 | 0.1666666666666643 | 0.5000000000000000 |
| 0.6666666666666643 | 0.3333333333333357 | 0.6666666666666643 |
| 0.6666666666666643 | 0.5000000000000000 | 0.8333333333333357 |
| 0.6666666666666643 | 0.6666666666666643 | 0.0000000000000000 |
| 0.6666666666666643 | 0.8333333333333357 | 0.1666666666666643 |
| 0.6666666666666643 | 0.0000000000000000 | 0.3333333333333357 |
| 0.8333333333333357 | 0.1666666666666643 | 0.6666666666666643 |
| 0.8333333333333357 | 0.3333333333333357 | 0.8333333333333357 |
| 0.8333333333333357 | 0.5000000000000000 | 0.0000000000000000 |
| 0.8333333333333357 | 0.6666666666666643 | 0.1666666666666643 |
| 0.8333333333333357 | 0.8333333333333357 | 0.3333333333333357 |
| 0.8333333333333357 | 0.0000000000000000 | 0.5000000000000000 |
| 0.0000000000000000 | 0.1666666666666643 | 0.8333333333333357 |
| 0.0000000000000000 | 0.3333333333333357 | 0.0000000000000000 |
| 0.0000000000000000 | 0.5000000000000000 | 0.1666666666666643 |
| 0.0000000000000000 | 0.6666666666666643 | 0.3333333333333357 |
| 0.0000000000000000 | 0.8333333333333357 | 0.5000000000000000 |
| 0.0000000000000000 | 0.0000000000000000 | 0.6666666666666643 |
| 0.3333333333333357 | 0.3333333333333357 | 0.0000000000000000 |
| 0.3333333333333357 | 0.5000000000000000 | 0.1666666666666643 |
| 0.3333333333333357 | 0.6666666666666643 | 0.3333333333333357 |
| 0.3333333333333357 | 0.8333333333333357 | 0.5000000000000000 |
| 0.3333333333333357 | 0.0000000000000000 | 0.6666666666666643 |

| | | |
|---|---|---|
| 0.3333333333333357 | 0.1666666666666643 | 0.8333333333333357 |
| 0.5000000000000000 | 0.3333333333333357 | 0.1666666666666643 |
| 0.5000000000000000 | 0.5000000000000000 | 0.3333333333333357 |
| 0.5000000000000000 | 0.6666666666666643 | 0.5000000000000000 |
| 0.5000000000000000 | 0.8333333333333357 | 0.6666666666666643 |
| 0.5000000000000000 | 0.0000000000000000 | 0.8333333333333357 |
| 0.5000000000000000 | 0.1666666666666643 | 0.0000000000000000 |
| 0.6666666666666643 | 0.3333333333333357 | 0.3333333333333357 |
| 0.6666666666666643 | 0.5000000000000000 | 0.5000000000000000 |
| 0.6666666666666643 | 0.6666666666666643 | 0.6666666666666643 |
| 0.6666666666666643 | 0.8333333333333357 | 0.8333333333333357 |
| 0.6666666666666643 | 0.0000000000000000 | 0.0000000000000000 |
| 0.6666666666666643 | 0.1666666666666643 | 0.1666666666666643 |
| 0.8333333333333357 | 0.3333333333333357 | 0.5000000000000000 |
| 0.8333333333333357 | 0.5000000000000000 | 0.6666666666666643 |
| 0.8333333333333357 | 0.6666666666666643 | 0.8333333333333357 |
| 0.8333333333333357 | 0.8333333333333357 | 0.0000000000000000 |
| 0.8333333333333357 | 0.0000000000000000 | 0.1666666666666643 |
| 0.8333333333333357 | 0.1666666666666643 | 0.3333333333333357 |
| 0.0000000000000000 | 0.3333333333333357 | 0.6666666666666643 |
| 0.0000000000000000 | 0.5000000000000000 | 0.8333333333333357 |
| 0.0000000000000000 | 0.6666666666666643 | 0.0000000000000000 |
| 0.0000000000000000 | 0.8333333333333357 | 0.1666666666666643 |
| 0.0000000000000000 | 0.0000000000000000 | 0.3333333333333357 |
| 0.0000000000000000 | 0.1666666666666643 | 0.5000000000000000 |
| 0.1666666666666643 | 0.3333333333333357 | 0.8333333333333357 |
| 0.1666666666666643 | 0.5000000000000000 | 0.0000000000000000 |
| 0.1666666666666643 | 0.6666666666666643 | 0.1666666666666643 |
| 0.1666666666666643 | 0.8333333333333357 | 0.3333333333333357 |
| 0.1666666666666643 | 0.0000000000000000 | 0.5000000000000000 |
| 0.1666666666666643 | 0.1666666666666643 | 0.6666666666666643 |
| 0.1666666666666643 | 0.1666666666666643 | 0.1666666666666643 |
| 0.1666666666666643 | 0.3333333333333357 | 0.3333333333333357 |
| 0.1666666666666643 | 0.5000000000000000 | 0.5000000000000000 |
| 0.1666666666666643 | 0.6666666666666643 | 0.6666666666666643 |
| 0.1666666666666643 | 0.8333333333333357 | 0.8333333333333357 |
| 0.1666666666666643 | 0.0000000000000000 | 0.0000000000000000 |
| 0.3333333333333357 | 0.1666666666666643 | 0.3333333333333357 |
| 0.3333333333333357 | 0.3333333333333357 | 0.5000000000000000 |
| 0.3333333333333357 | 0.5000000000000000 | 0.6666666666666643 |
| 0.3333333333333357 | 0.6666666666666643 | 0.8333333333333357 |
| 0.3333333333333357 | 0.8333333333333357 | 0.0000000000000000 |
| 0.3333333333333357 | 0.0000000000000000 | 0.1666666666666643 |
| 0.5000000000000000 | 0.1666666666666643 | 0.5000000000000000 |
| 0.5000000000000000 | 0.3333333333333357 | 0.6666666666666643 |
| 0.5000000000000000 | 0.5000000000000000 | 0.8333333333333357 |
| 0.5000000000000000 | 0.6666666666666643 | 0.0000000000000000 |
| 0.5000000000000000 | 0.8333333333333357 | 0.1666666666666643 |
| 0.5000000000000000 | 0.0000000000000000 | 0.3333333333333357 |
| 0.6666666666666643 | 0.1666666666666643 | 0.6666666666666643 |
| 0.6666666666666643 | 0.3333333333333357 | 0.8333333333333357 |
| 0.6666666666666643 | 0.5000000000000000 | 0.0000000000000000 |
| 0.6666666666666643 | 0.6666666666666643 | 0.1666666666666643 |
| 0.6666666666666643 | 0.8333333333333357 | 0.3333333333333357 |
| 0.6666666666666643 | 0.0000000000000000 | 0.5000000000000000 |
| 0.8333333333333357 | 0.1666666666666643 | 0.8333333333333357 |
| 0.8333333333333357 | 0.3333333333333357 | 0.0000000000000000 |
| 0.8333333333333357 | 0.5000000000000000 | 0.1666666666666643 |

| | | |
|---|---|---|
| 0.8333333333333357 | 0.6666666666666643 | 0.3333333333333357 |
| 0.8333333333333357 | 0.8333333333333357 | 0.5000000000000000 |
| 0.8333333333333357 | 0.0000000000000000 | 0.6666666666666643 |
| 0.0000000000000000 | 0.1666666666666643 | 0.0000000000000000 |
| 0.0000000000000000 | 0.3333333333333357 | 0.1666666666666643 |
| 0.0000000000000000 | 0.5000000000000000 | 0.3333333333333357 |
| 0.0000000000000000 | 0.6666666666666643 | 0.5000000000000000 |
| 0.0000000000000000 | 0.8333333333333357 | 0.6666666666666643 |
| 0.0000000000000000 | 0.0000000000000000 | 0.8333333333333357 |
| 0.3333333333333357 | 0.3333333333333357 | 0.1666666666666643 |
| 0.3333333333333357 | 0.5000000000000000 | 0.3333333333333357 |
| 0.3333333333333357 | 0.6666666666666643 | 0.5000000000000000 |
| 0.3333333333333357 | 0.8333333333333357 | 0.6666666666666643 |
| 0.3333333333333357 | 0.0000000000000000 | 0.8333333333333357 |
| 0.3333333333333357 | 0.1666666666666643 | 0.0000000000000000 |
| 0.5000000000000000 | 0.3333333333333357 | 0.3333333333333357 |
| 0.5000000000000000 | 0.6666666666666643 | 0.6666666666666643 |
| 0.5000000000000000 | 0.8333333333333357 | 0.8333333333333357 |
| 0.5000000000000000 | 0.0000000000000000 | 0.0000000000000000 |
| 0.5000000000000000 | 0.1666666666666643 | 0.1666666666666643 |
| 0.6666666666666643 | 0.3333333333333357 | 0.5000000000000000 |
| 0.6666666666666643 | 0.5000000000000000 | 0.6666666666666643 |
| 0.6666666666666643 | 0.6666666666666643 | 0.8333333333333357 |
| 0.6666666666666643 | 0.8333333333333357 | 0.0000000000000000 |
| 0.6666666666666643 | 0.0000000000000000 | 0.1666666666666643 |
| 0.6666666666666643 | 0.1666666666666643 | 0.3333333333333357 |
| 0.8333333333333357 | 0.3333333333333357 | 0.6666666666666643 |
| 0.8333333333333357 | 0.5000000000000000 | 0.8333333333333357 |
| 0.8333333333333357 | 0.6666666666666643 | 0.0000000000000000 |
| 0.8333333333333357 | 0.8333333333333357 | 0.1666666666666643 |
| 0.8333333333333357 | 0.0000000000000000 | 0.3333333333333357 |
| 0.8333333333333357 | 0.1666666666666643 | 0.5000000000000000 |
| 0.0000000000000000 | 0.3333333333333357 | 0.8333333333333357 |
| 0.0000000000000000 | 0.5000000000000000 | 0.0000000000000000 |
| 0.0000000000000000 | 0.6666666666666643 | 0.1666666666666643 |
| 0.0000000000000000 | 0.8333333333333357 | 0.3333333333333357 |
| 0.0000000000000000 | 0.0000000000000000 | 0.5000000000000000 |
| 0.0000000000000000 | 0.1666666666666643 | 0.6666666666666643 |
| 0.1666666666666643 | 0.3333333333333357 | 0.0000000000000000 |
| 0.1666666666666643 | 0.5000000000000000 | 0.1666666666666643 |
| 0.1666666666666643 | 0.6666666666666643 | 0.3333333333333357 |
| 0.1666666666666643 | 0.8333333333333357 | 0.5000000000000000 |
| 0.1666666666666643 | 0.0000000000000000 | 0.6666666666666643 |
| 0.1666666666666643 | 0.1666666666666643 | 0.8333333333333357 |
| 0.5000000000000000 | 0.5000000000000000 | 0.1666666666666643 |
| 0.5000000000000000 | 0.6666666666666643 | 0.3333333333333357 |
| 0.5000000000000000 | 0.8333333333333357 | 0.5000000000000000 |
| 0.5000000000000000 | 0.0000000000000000 | 0.6666666666666643 |
| 0.5000000000000000 | 0.1666666666666643 | 0.8333333333333357 |
| 0.5000000000000000 | 0.3333333333333357 | 0.0000000000000000 |
| 0.6666666666666643 | 0.5000000000000000 | 0.3333333333333357 |
| 0.6666666666666643 | 0.6666666666666643 | 0.5000000000000000 |
| 0.6666666666666643 | 0.8333333333333357 | 0.6666666666666643 |
| 0.6666666666666643 | 0.0000000000000000 | 0.8333333333333357 |
| 0.6666666666666643 | 0.1666666666666643 | 0.0000000000000000 |
| 0.6666666666666643 | 0.3333333333333357 | 0.1666666666666643 |
| 0.8333333333333357 | 0.5000000000000000 | 0.5000000000000000 |
| 0.8333333333333357 | 0.6666666666666643 | 0.6666666666666643 |

```
  0.8333333333333357  0.8333333333333357  0.8333333333333357
  0.8333333333333357  0.0000000000000000  0.0000000000000000
  0.8333333333333357  0.1666666666666643  0.1666666666666643
  0.8333333333333357  0.3333333333333357  0.3333333333333357
  0.0000000000000000  0.5000000000000000  0.6666666666666643
  0.0000000000000000  0.6666666666666643  0.8333333333333357
  0.0000000000000000  0.8333333333333357  0.0000000000000000
  0.0000000000000000  0.0000000000000000  0.1666666666666643
  0.0000000000000000  0.1666666666666643  0.3333333333333357
  0.0000000000000000  0.3333333333333357  0.5000000000000000
  0.1666666666666643  0.5000000000000000  0.8333333333333357
  0.1666666666666643  0.6666666666666643  0.0000000000000000
  0.1666666666666643  0.8333333333333357  0.1666666666666643
  0.1666666666666643  0.0000000000000000  0.3333333333333357
  0.1666666666666643  0.1666666666666643  0.5000000000000000
  0.1666666666666643  0.3333333333333357  0.6666666666666643
  0.3333333333333357  0.5000000000000000  0.0000000000000000
  0.3333333333333357  0.6666666666666643  0.1666666666666643
  0.3333333333333357  0.8333333333333357  0.3333333333333357
  0.3333333333333357  0.0000000000000000  0.5000000000000000
  0.3333333333333357  0.1666666666666643  0.6666666666666643
  0.3333333333333357  0.3333333333333357  0.8333333333333357
  0.5000000000000000  0.5000000000000000  0.5000000000000000
```

### H. NaCl with Na impurity (relaxed using DFT-PBE)

Hartree-Fock energy: −1377.351 eV.

```
LiCl with Na impurity (relaxed)
   1.00000000000000
     15.4731335457707697    0.0000000000000000    0.0000000000000000
      0.0000000000000000   15.4731335457707697    0.0000000000000000
      0.0000000000000000    0.0000000000000000   15.4731335457707697
   Cl    Li    Na
   108   107   1
Direct
  0.0000000000000000  0.0000000000000000  0.0000000000000000
  0.0000000000000000  0.1666585195992951  0.1666585195992951
  0.0000000000000000  0.3332160505555848  0.3332160505555848
  0.0000000000000000  0.5000000000000000  0.5000000000000000
  0.0000000000000000  0.6667839494444152  0.6667839494444152
  0.0000000000000000  0.8333414804007049  0.8333414804007049
  0.1666585195992951  0.0000000000000000  0.1666585195992951
  0.1666757492549067  0.1666757492549067  0.3331837283210533
  0.1656884229987057  0.3324287124798815  0.5000000000000000
  0.1656884229987057  0.5000000000000000  0.6675712875201185
  0.1666757492549067  0.6668162716789467  0.8333242507450933
  0.1666585195992951  0.8333414804007049  0.0000000000000000
  0.3332160505555848  0.0000000000000000  0.3332160505555848
  0.3324287124798815  0.1656884229987057  0.5000000000000000
  0.3335099581584444  0.3335099581584444  0.6664900418415556
  0.3324287124798815  0.5000000000000000  0.8343115770012943
  0.3332160505555848  0.6667839494444152  0.0000000000000000
  0.3331837283210533  0.8333242507450933  0.1666757492549067
  0.5000000000000000  0.0000000000000000  0.5000000000000000
  0.5000000000000000  0.1656884229987057  0.6675712875201185
  0.5000000000000000  0.3324287124798815  0.8343115770012943
```

| | | |
|---|---|---|
| 0.5000000000000000 | 0.5000000000000000 | 0.0000000000000000 |
| 0.5000000000000000 | 0.6675712875201185 | 0.1656884229987057 |
| 0.5000000000000000 | 0.8343115770012943 | 0.3324287124798815 |
| 0.6667839494444152 | 0.0000000000000000 | 0.6667839494444152 |
| 0.6668162716789467 | 0.1666757492549067 | 0.8333242507450933 |
| 0.6667839494444152 | 0.3332160505555848 | 0.0000000000000000 |
| 0.6675712875201185 | 0.5000000000000000 | 0.1656884229987057 |
| 0.6664900418415556 | 0.6664900418415556 | 0.3335099581584444 |
| 0.6675712875201185 | 0.8343115770012943 | 0.5000000000000000 |
| 0.8333414804007049 | 0.0000000000000000 | 0.8333414804007049 |
| 0.8333414804007049 | 0.1666585195992951 | 0.0000000000000000 |
| 0.8333242507450933 | 0.3331837283210533 | 0.1666757492549067 |
| 0.8343115770012943 | 0.5000000000000000 | 0.3324287124798815 |
| 0.8343115770012943 | 0.6675712875201185 | 0.5000000000000000 |
| 0.8333242507450933 | 0.8333242507450933 | 0.6668162716789467 |
| 0.1666585195992951 | 0.1666585195992951 | 0.0000000000000000 |
| 0.1666757492549067 | 0.3331837283210533 | 0.1666757492549067 |
| 0.1656884229987057 | 0.5000000000000000 | 0.3324287124798815 |
| 0.1656884229987057 | 0.6675712875201185 | 0.5000000000000000 |
| 0.1666757492549067 | 0.8333242507450933 | 0.6668162716789467 |
| 0.1666585195992951 | 0.0000000000000000 | 0.8333414804007049 |
| 0.3331837283210533 | 0.1666757492549067 | 0.1666757492549067 |
| 0.3335099581584444 | 0.3335099581584444 | 0.3335099581584444 |
| 0.3258976365508843 | 0.5000000000000000 | 0.5000000000000000 |
| 0.3335099581584444 | 0.6664900418415556 | 0.6664900418415556 |
| 0.3331837283210533 | 0.8333242507450933 | 0.8333242507450933 |
| 0.3332298888154881 | 0.0000000000000000 | 0.0000000000000000 |
| 0.5000000000000000 | 0.1656884229987057 | 0.3324287124798815 |
| 0.5000000000000000 | 0.3258976365508843 | 0.5000000000000000 |
| 0.5000000000000000 | 0.5000000000000000 | 0.6741023634491157 |
| 0.5000000000000000 | 0.6675712875201185 | 0.8343115770012943 |
| 0.5000000000000000 | 0.8337128017732169 | 0.0000000000000000 |
| 0.5000000000000000 | 0.0000000000000000 | 0.1662871982267831 |
| 0.6675712875201185 | 0.1656884229987057 | 0.5000000000000000 |
| 0.6664900418415556 | 0.3335099581584444 | 0.6664900418415556 |
| 0.6675712875201185 | 0.5000000000000000 | 0.8343115770012943 |
| 0.6667839494444152 | 0.6667839494444152 | 0.0000000000000000 |
| 0.6668162716789467 | 0.8333242507450933 | 0.1666757492549067 |
| 0.6667839494444152 | 0.0000000000000000 | 0.3332160505555848 |
| 0.8333242507450933 | 0.1666757492549067 | 0.6668162716789467 |
| 0.8333242507450933 | 0.3331837283210533 | 0.8333242507450933 |
| 0.8337128017732169 | 0.5000000000000000 | 0.0000000000000000 |
| 0.8333242507450933 | 0.6668162716789467 | 0.1666757492549067 |
| 0.8333242507450933 | 0.8333242507450933 | 0.3331837283210533 |
| 0.8337128017732169 | 0.0000000000000000 | 0.5000000000000000 |
| 0.0000000000000000 | 0.1666585195992951 | 0.8333414804007049 |
| 0.0000000000000000 | 0.3332298888154881 | 0.0000000000000000 |
| 0.0000000000000000 | 0.5000000000000000 | 0.1662871982267831 |
| 0.0000000000000000 | 0.6667839494444152 | 0.3332160505555848 |
| 0.0000000000000000 | 0.8337128017732169 | 0.5000000000000000 |
| 0.0000000000000000 | 0.0000000000000000 | 0.6667701111845119 |
| 0.3332160505555848 | 0.3332160505555848 | 0.0000000000000000 |
| 0.3324287124798815 | 0.5000000000000000 | 0.1656884229987057 |
| 0.3335099581584444 | 0.6664900418415556 | 0.3335099581584444 |
| 0.3324287124798815 | 0.8343115770012943 | 0.5000000000000000 |
| 0.3332160505555848 | 0.0000000000000000 | 0.6667839494444152 |
| 0.3331837283210533 | 0.1666757492549067 | 0.8333242507450933 |
| 0.5000000000000000 | 0.3324287124798815 | 0.1656884229987057 |

| | | |
|---|---|---|
| 0.5000000000000000 | 0.5000000000000000 | 0.3258976365508843 |
| 0.5000000000000000 | 0.6741023634491157 | 0.5000000000000000 |
| 0.5000000000000000 | 0.8343115770012943 | 0.6675712875201185 |
| 0.5000000000000000 | 0.0000000000000000 | 0.8337128017732169 |
| 0.5000000000000000 | 0.1662871982267831 | 0.0000000000000000 |
| 0.6664900418415556 | 0.3335099581584444 | 0.3335099581584444 |
| 0.6741023634491157 | 0.5000000000000000 | 0.5000000000000000 |
| 0.6664900418415556 | 0.6664900418415556 | 0.6664900418415556 |
| 0.6668162716789467 | 0.8333242507450933 | 0.8333242507450933 |
| 0.6667701111845119 | 0.0000000000000000 | 0.0000000000000000 |
| 0.6668162716789467 | 0.1666757492549067 | 0.1666757492549067 |
| 0.8343115770012943 | 0.3324287124798815 | 0.5000000000000000 |
| 0.8343115770012943 | 0.5000000000000000 | 0.6675712875201185 |
| 0.8333242507450933 | 0.6668162716789467 | 0.8333242507450933 |
| 0.8333414804007049 | 0.8333414804007049 | 0.0000000000000000 |
| 0.8333414804007049 | 0.0000000000000000 | 0.1666585195992951 |
| 0.8333242507450933 | 0.1666757492549067 | 0.3331837283210533 |
| 0.0000000000000000 | 0.3332160505555848 | 0.6667839494444152 |
| 0.0000000000000000 | 0.5000000000000000 | 0.8337128017732169 |
| 0.0000000000000000 | 0.6667701111845119 | 0.0000000000000000 |
| 0.0000000000000000 | 0.8333414804007049 | 0.1666585195992951 |
| 0.0000000000000000 | 0.0000000000000000 | 0.3332298888154881 |
| 0.0000000000000000 | 0.1662871982267831 | 0.5000000000000000 |
| 0.1666757492549067 | 0.3331837283210533 | 0.8333242507450933 |
| 0.1662871982267831 | 0.5000000000000000 | 0.0000000000000000 |
| 0.1666757492549067 | 0.6668162716789467 | 0.1666757492549067 |
| 0.1666757492549067 | 0.8333242507450933 | 0.3331837283210533 |
| 0.1662871982267831 | 0.0000000000000000 | 0.5000000000000000 |
| 0.1666757492549067 | 0.1666757492549067 | 0.6668162716789467 |
| 0.1666166411625198 | 0.1666166411625198 | 0.1666166411625198 |
| 0.1663136706418271 | 0.3332222026247038 | 0.3332222026247038 |
| 0.1648485681328609 | 0.5000000000000000 | 0.5000000000000000 |
| 0.1663136706418271 | 0.6667777973752962 | 0.6667777973752962 |
| 0.1666166411625198 | 0.8333833588374802 | 0.8333833588374802 |
| 0.1666343657448337 | 0.0000000000000000 | 0.0000000000000000 |
| 0.3332222026247038 | 0.1663136706418271 | 0.3332222026247038 |
| 0.3315795677868962 | 0.3315795677868962 | 0.5000000000000000 |
| 0.3315795677868962 | 0.5000000000000000 | 0.6684204322131038 |
| 0.3332222026247038 | 0.6667777973752962 | 0.8336863293581729 |
| 0.3333220897590365 | 0.8334123031924534 | 0.0000000000000000 |
| 0.3333220897590365 | 0.0000000000000000 | 0.1665876968075466 |
| 0.5000000000000000 | 0.1648485681328609 | 0.5000000000000000 |
| 0.5000000000000000 | 0.3315795677868962 | 0.6684204322131038 |
| 0.5000000000000000 | 0.5000000000000000 | 0.8351514318671391 |
| 0.5000000000000000 | 0.6672523251784455 | 0.0000000000000000 |
| 0.5000000000000000 | 0.8336761101727248 | 0.1663238898272752 |
| 0.5000000000000000 | 0.0000000000000000 | 0.3327476748215545 |
| 0.6667777973752962 | 0.1663136706418271 | 0.6667777973752962 |
| 0.6667777973752962 | 0.3332222026247038 | 0.8336863293581729 |
| 0.6672523251784455 | 0.5000000000000000 | 0.0000000000000000 |
| 0.6667777973752962 | 0.6667777973752962 | 0.1663136706418271 |
| 0.6667777973752962 | 0.8336863293581729 | 0.3332222026247038 |
| 0.6672523251784455 | 0.0000000000000000 | 0.5000000000000000 |
| 0.8333833588374802 | 0.1666166411625198 | 0.8333833588374802 |
| 0.8334123031924534 | 0.3333220897590365 | 0.0000000000000000 |
| 0.8336761101727248 | 0.5000000000000000 | 0.1663238898272752 |
| 0.8336863293581729 | 0.6667777973752962 | 0.3332222026247038 |
| 0.8336761101727248 | 0.8336761101727248 | 0.5000000000000000 |

| | | |
|---|---|---|
| 0.8334123031924534 | 0.0000000000000000 | 0.6666779102409635 |
| 0.0000000000000000 | 0.1666343657448337 | 0.0000000000000000 |
| 0.0000000000000000 | 0.3333220897590365 | 0.1665876968075466 |
| 0.0000000000000000 | 0.5000000000000000 | 0.3327476748215545 |
| 0.0000000000000000 | 0.6672523251784455 | 0.5000000000000000 |
| 0.0000000000000000 | 0.8334123031924534 | 0.6666779102409635 |
| 0.0000000000000000 | 0.0000000000000000 | 0.8333656342551663 |
| 0.3332222026247038 | 0.3332222026247038 | 0.1663136706418271 |
| 0.3315795677868962 | 0.5000000000000000 | 0.3315795677868962 |
| 0.3315795677868962 | 0.6684204322131038 | 0.5000000000000000 |
| 0.3332222026247038 | 0.8336863293581729 | 0.6667777973752962 |
| 0.3333220897590365 | 0.0000000000000000 | 0.8334123031924534 |
| 0.3333220897590365 | 0.1665876968075466 | 0.0000000000000000 |
| 0.5000000000000000 | 0.3315795677868962 | 0.3315795677868962 |
| 0.5000000000000000 | 0.6684204322131038 | 0.6684204322131038 |
| 0.5000000000000000 | 0.8336761101727248 | 0.8336761101727248 |
| 0.5000000000000000 | 0.0000000000000000 | 0.0000000000000000 |
| 0.5000000000000000 | 0.1663238898272752 | 0.1663238898272752 |
| 0.6684204322131038 | 0.3315795677868962 | 0.5000000000000000 |
| 0.6684204322131038 | 0.5000000000000000 | 0.6684204322131038 |
| 0.6667777973752962 | 0.6667777973752962 | 0.8336863293581729 |
| 0.6666779102409635 | 0.8334123031924534 | 0.0000000000000000 |
| 0.6666779102409635 | 0.0000000000000000 | 0.1665876968075466 |
| 0.6667777973752962 | 0.1663136706418271 | 0.3332222026247038 |
| 0.8336863293581729 | 0.3332222026247038 | 0.6667777973752962 |
| 0.8336761101727248 | 0.5000000000000000 | 0.8336761101727248 |
| 0.8334123031924534 | 0.6666779102409635 | 0.0000000000000000 |
| 0.8333833588374802 | 0.8333833588374802 | 0.1666166411625198 |
| 0.8334123031924534 | 0.0000000000000000 | 0.3333220897590365 |
| 0.8336761101727248 | 0.1663238898272752 | 0.5000000000000000 |
| 0.0000000000000000 | 0.3333220897590365 | 0.8334123031924534 |
| 0.0000000000000000 | 0.5000000000000000 | 0.0000000000000000 |
| 0.0000000000000000 | 0.6666779102409635 | 0.1665876968075466 |
| 0.0000000000000000 | 0.8334123031924534 | 0.3333220897590365 |
| 0.0000000000000000 | 0.0000000000000000 | 0.5000000000000000 |
| 0.0000000000000000 | 0.1665876968075466 | 0.6666779102409635 |
| 0.1665876968075466 | 0.3333220897590365 | 0.0000000000000000 |
| 0.1663238898272752 | 0.5000000000000000 | 0.1663238898272752 |
| 0.1663136706418271 | 0.6667777973752962 | 0.3332222026247038 |
| 0.1663238898272752 | 0.8336761101727248 | 0.5000000000000000 |
| 0.1665876968075466 | 0.0000000000000000 | 0.6666779102409635 |
| 0.1666166411625198 | 0.1666166411625198 | 0.8333833588374802 |
| 0.5000000000000000 | 0.5000000000000000 | 0.1648485681328609 |
| 0.5000000000000000 | 0.6684204322131038 | 0.3315795677868962 |
| 0.5000000000000000 | 0.8351514318671391 | 0.5000000000000000 |
| 0.5000000000000000 | 0.0000000000000000 | 0.6672523251784455 |
| 0.5000000000000000 | 0.1663238898272752 | 0.8336761101727248 |
| 0.5000000000000000 | 0.3327476748215545 | 0.0000000000000000 |
| 0.6684204322131038 | 0.5000000000000000 | 0.3315795677868962 |
| 0.6684204322131038 | 0.6684204322131038 | 0.5000000000000000 |
| 0.6667777973752962 | 0.8336863293581729 | 0.6667777973752962 |
| 0.6666779102409635 | 0.0000000000000000 | 0.8334123031924534 |
| 0.6666779102409635 | 0.1665876968075466 | 0.0000000000000000 |
| 0.6667777973752962 | 0.3332222026247038 | 0.1663136706418271 |
| 0.8351514318671391 | 0.5000000000000000 | 0.5000000000000000 |
| 0.8336863293581729 | 0.6667777973752962 | 0.6667777973752962 |
| 0.8333833588374802 | 0.8333833588374802 | 0.8333833588374802 |
| 0.8333656342551663 | 0.0000000000000000 | 0.0000000000000000 |

| | | |
|---|---|---|
| 0.8333833588374802 | 0.1666166411625198 | 0.1666166411625198 |
| 0.8336863293581729 | 0.3332222026247038 | 0.3332222026247038 |
| 0.0000000000000000 | 0.5000000000000000 | 0.6672523251784455 |
| 0.0000000000000000 | 0.6666779102409635 | 0.8334123031924534 |
| 0.0000000000000000 | 0.8333656342551663 | 0.0000000000000000 |
| 0.0000000000000000 | 0.0000000000000000 | 0.1666343657448337 |
| 0.0000000000000000 | 0.1665876968075466 | 0.3333220897590365 |
| 0.0000000000000000 | 0.3327476748215545 | 0.5000000000000000 |
| 0.1663238898272752 | 0.5000000000000000 | 0.8336761101727248 |
| 0.1665876968075466 | 0.6666779102409635 | 0.0000000000000000 |
| 0.1666166411625198 | 0.8333833588374802 | 0.1666166411625198 |
| 0.1665876968075466 | 0.0000000000000000 | 0.3333220897590365 |
| 0.1663238898272752 | 0.1663238898272752 | 0.5000000000000000 |
| 0.1663136706418271 | 0.3332222026247038 | 0.6667777973752962 |
| 0.3327476748215545 | 0.5000000000000000 | 0.0000000000000000 |
| 0.3332222026247038 | 0.6667777973752962 | 0.1663136706418271 |
| 0.3332222026247038 | 0.8336863293581729 | 0.3332222026247038 |
| 0.3327476748215545 | 0.0000000000000000 | 0.5000000000000000 |
| 0.3332222026247038 | 0.1663136706418271 | 0.6667777973752962 |
| 0.3332222026247038 | 0.3332222026247038 | 0.8336863293581729 |
| 0.5000000000000000 | 0.5000000000000000 | 0.5000000000000000 |


[1] A. Grüneis, G. H. Booth, M. Marsman, J. Spencer, A. Alavi, and G. Kresse, J. Chem. Theory Comput. **7**, 2780 (2011).

[2] F. Hummel, T. Tsatsoulis, and A. Grüneis, The Journal of Chemical Physics **146**, 124105 (2017), https://doi.org/10.1063/1.4977994.
